# Supplementary material for: Unsupervised Anomaly Localization using Variational Auto-Encoders
Source: arXiv:1907.02796 source file (2019-07-11)

## ISLES 15

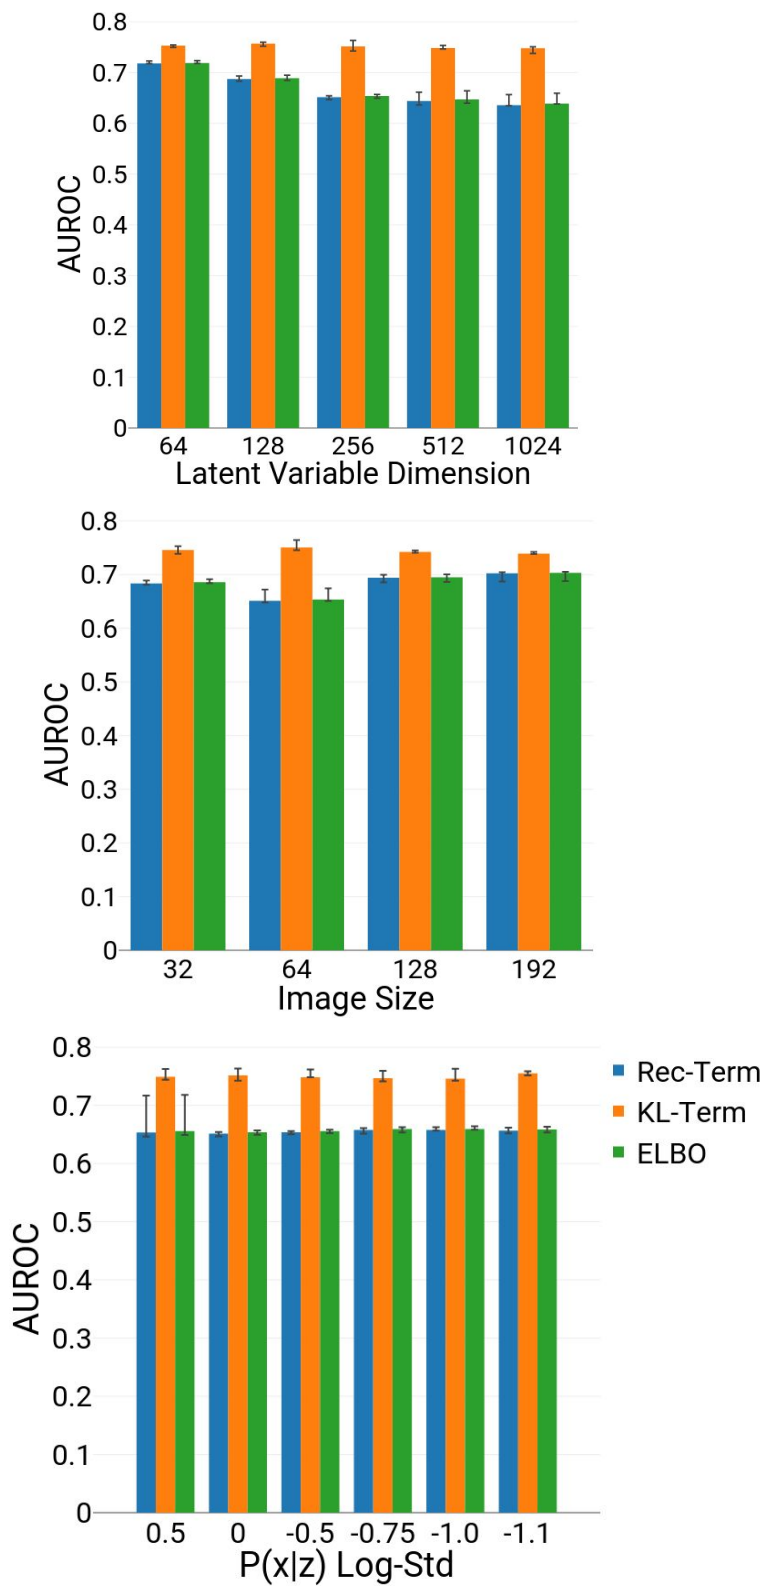

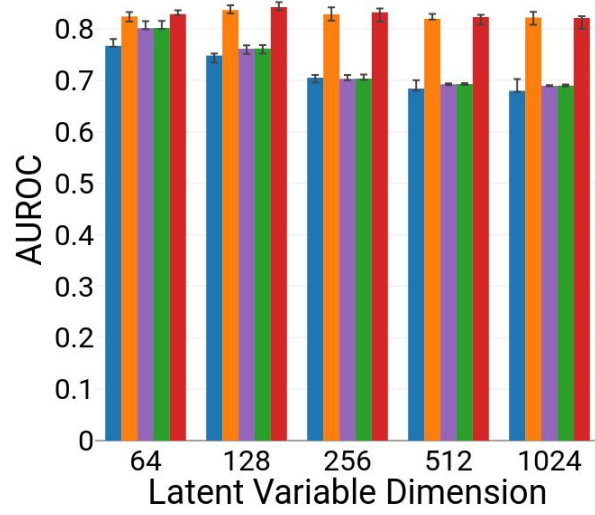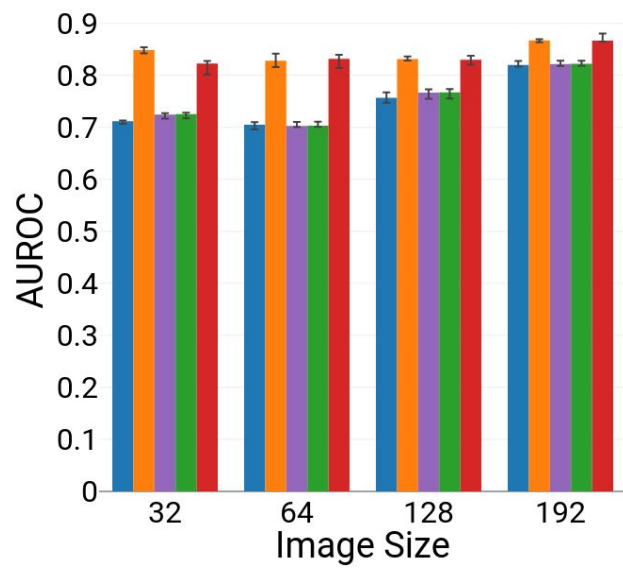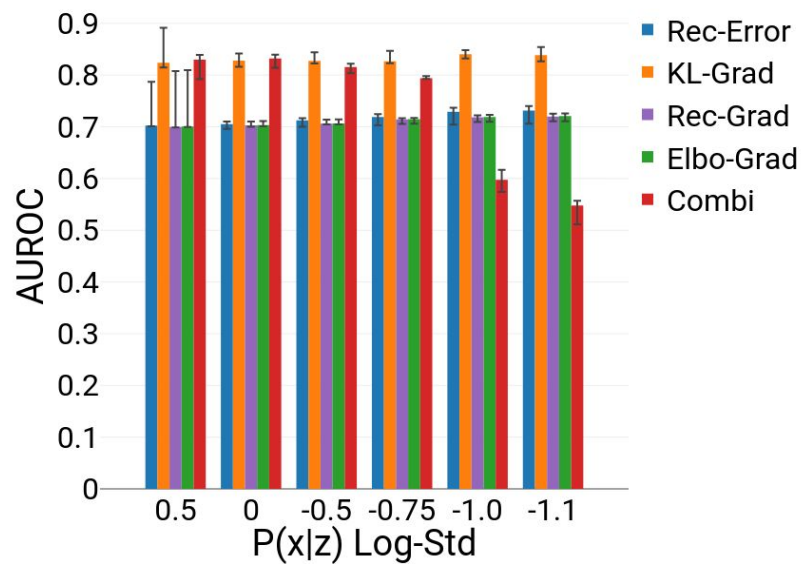

Supplement: Supplementary file 1 [file supplement1_isles.pdf]
