# Supplementary material for: Unsupervised Anomaly Localization using Variational Auto-Encoders
Source: arXiv:1907.02796 source file (2019-07-11)

## 2D Example & Visualizations

Gaussian Mixture

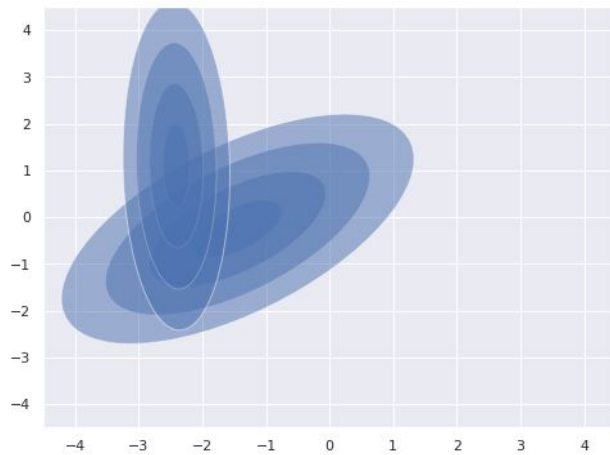

Samples

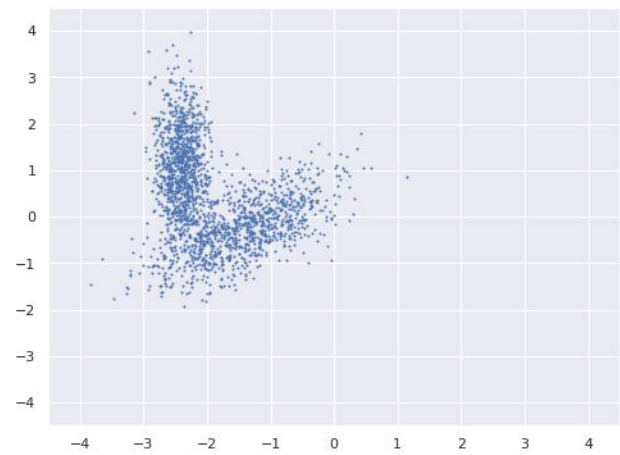

Density - Heatmap

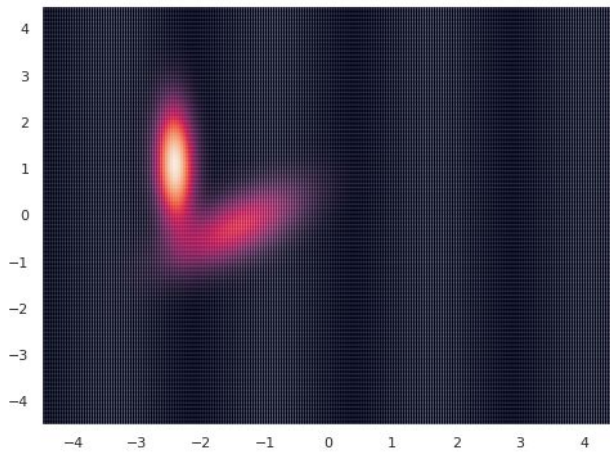

$$\frac{\partial p(x)}{\partial x}$$

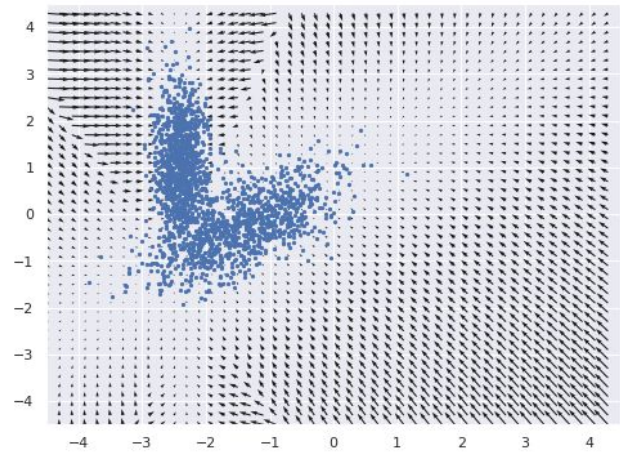

VAE - Trained on  
Gaussian Mixture

Samples:

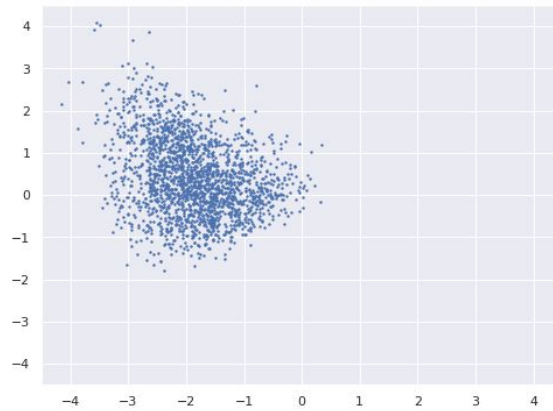

ELBO - Heatmap:

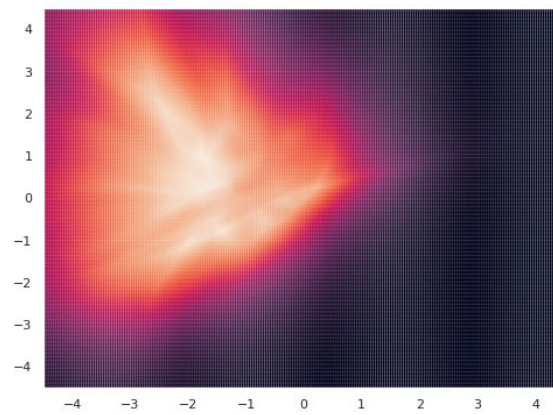

KL-Term - Heatmap:

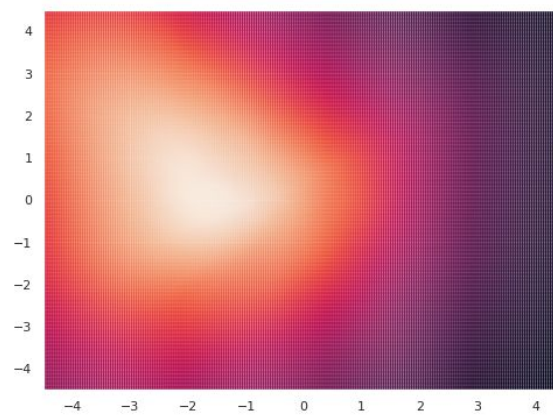

Rec-Term Heatmap:

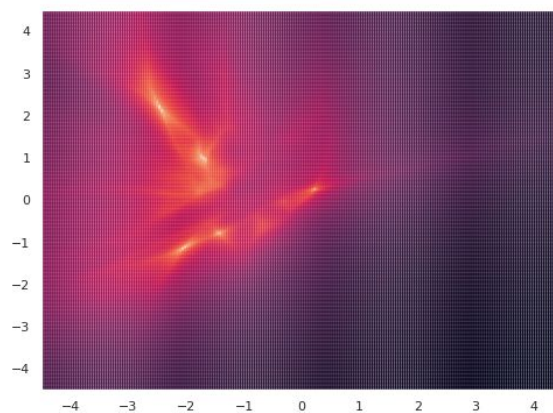

ELBO - Gradients:

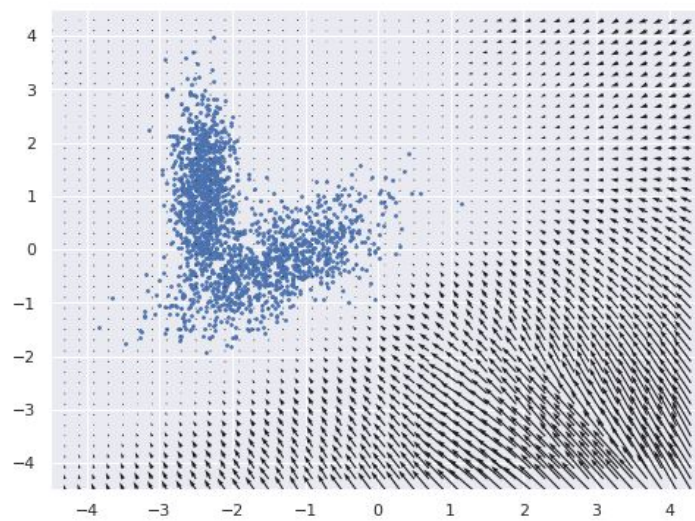

KL-Term Gradients:

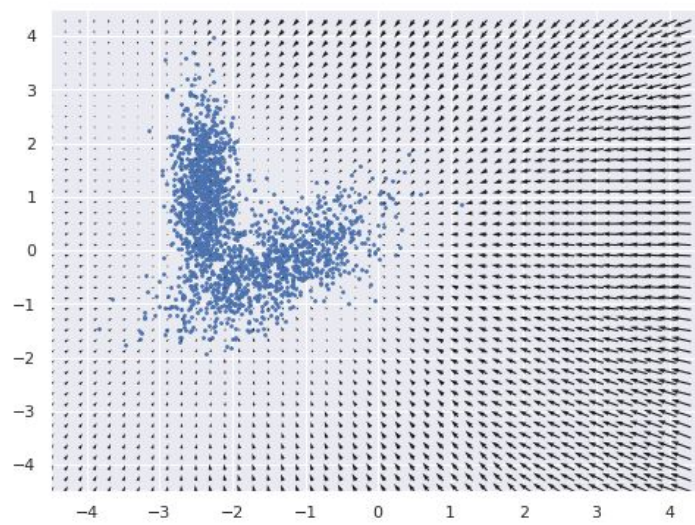

Rec-Term Gradients:

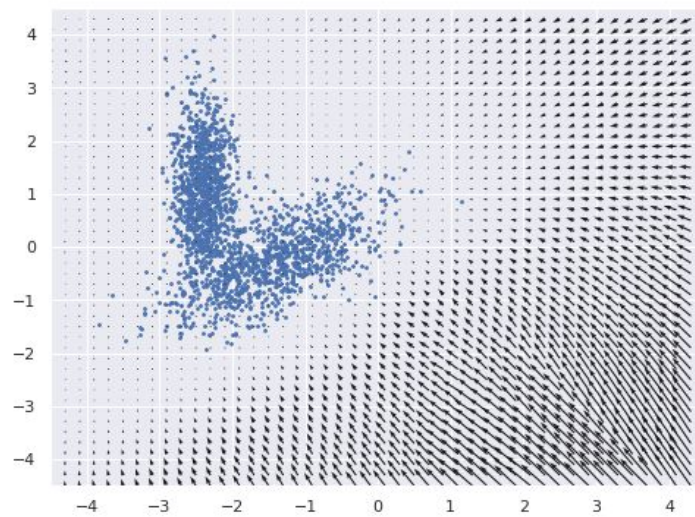



*Gradient Norm:*

ELBO-Gradient magnitude:

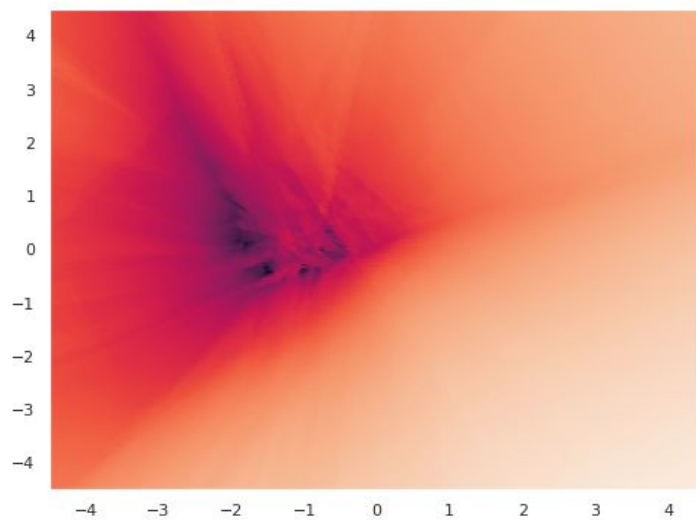

KL-Gradient magnitude:

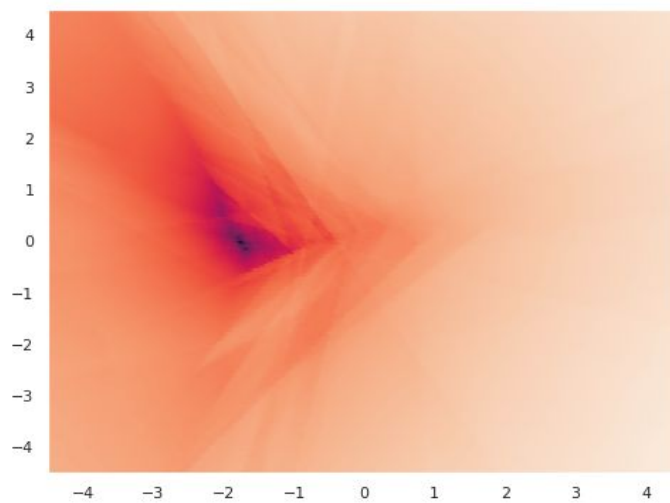

Rec-Gradient magnitude:

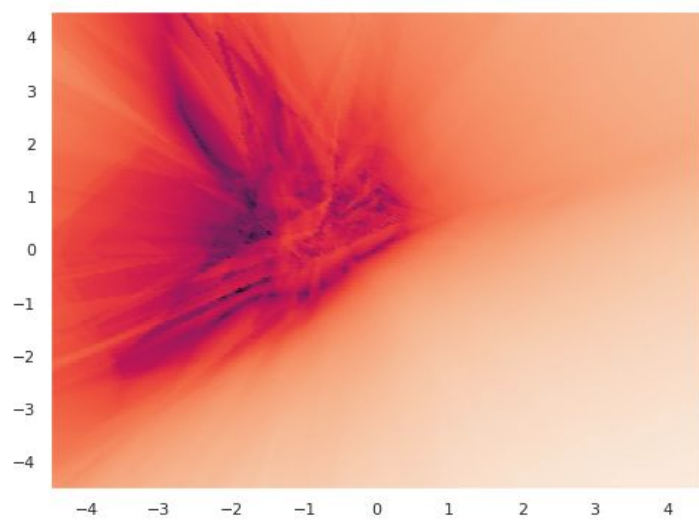

Supplement: Supplementary file 2 [file supplement2_2d_example.pdf]
